# Supplementary material for: FusionQ: A Generic and Optimal Decoding Framework for Ultra-Low-Latency Quantum Error Correction
Source: arXiv:2611.13111 source file (2026-11-09)
Supplement: Supplementary file 1 [file Appendix.tex]

\section{Data}
